# Supplementary material for: Van der Waals-Driven Network Restructuring Explains Time-Dependent Piezoresistivity in Soft Nanocomposites
Source: arXiv:2505.11506 ancillary file (2025-05-02)
Supplement: Supplementary file 1 [file supplementary.pdf]

# Supplementary Materials

Logan Ritchie[1], Elke Pahl[2,3], and Iain Anderson[1]

[1]Biomimetics Laboratory, Auckland Bioengineering Institute, The University of Auckland, Auckland, New Zealand
[2]MacDiarmid Institute for Advanced Materials and Nanotechnology, Wellington, New Zealand
[3]Department of Physics, The University of Auckland, Auckland, New Zealand

## Note

This document provides supplementary information in support of the manuscript titled:
*"Van der Waals–Driven Network Restructuring Explains Time-Dependent Piezoresistivity in Soft Nanocomposites"*

## 1 Comparison of van der Waals forces to viscoelastic stresses

The Everaers interaction describes the potential energy of interaction between two particles due to van der Waals attractions and rigidity [1]. Equation 1 represents the interaction between two identical spherical particles.

$$\begin{aligned} U_{\mathrm{vdw}} = & \frac{A}{37800}\frac{\sigma_{LJ}^6}{r}\left(\frac{r^2-14Rr+54R^2}{(r-2R)^7}+\frac{r^2+14Rr+54R^2}{(r+2R)^7}-\frac{2r^2-60R^2}{r^7}\right) \\ & -\frac{A}{6}\left(\frac{2R^2}{r^2-4R^2}+\frac{2R^2}{r^2}+\ln\frac{r^2-4R^2}{r^2}\right) \end{aligned} \tag{1}$$

Where $U_{\mathrm{vdw}}$ is potential energy, $A$ is the Hamaker constant, $\sigma_{LJ}$ is the characteristic Lennard Jones length, $r$ is the distance between particle centres, and $R$ is the radius of the particles. The two material variables needed in order to represent this equation correctly are the Hamaker constant $A$, and the radius of the particles $R$.

From electron microscope imaging, the radius of the primary particles of typical carbon blacks ranges from 5 nm – 50 nm [2]. Unfortunately, an exact measurement of the Hamaker constant for these materials is more challenging to obtain. Furthermore, the Hamaker constant depends not only on the filler materials, but also on the medium within which the particles are embedded [3]. However, it is known that for any medium, the nature of this interaction is that it will always be attractive between two particles of the same material [4]. It is known that the typical value of the Hamaker constant for many materials is on the order of magnitude of $1 \times 10^{-19}$ J [4], and indeed this is the case for carbon black dispersed in various media [3].

Figure 1 shows the Everaers potential with a Hamaker constant of $1 \times 10^{-19}$ J, for spherical particles with radii ranging from 5 – 100 nm.

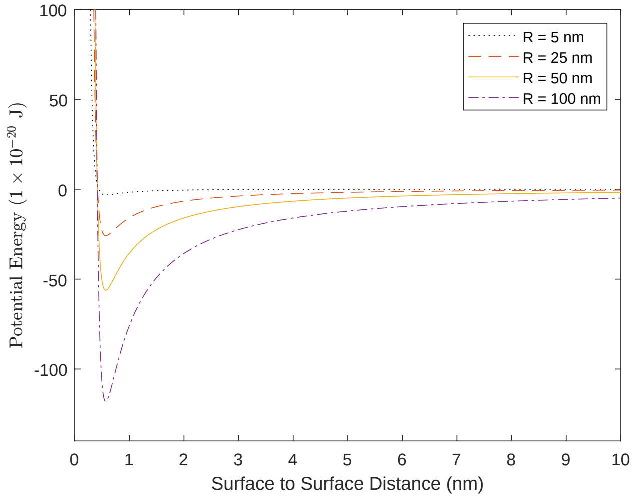


Figure 1: Everaers Potential - potential energy of interaction between two spherical particles with radii $R$ and Hamaker constant $1 \times 10^{-19}$ J

By taking the negative of the derivative of the van der Waals potential with respect to distance $r$, we can calculate the force acting between two particles due to the van der Waals interactions (Equation 2).

$$\begin{aligned} F = {} & \frac{A\sigma^2}{37800}\frac{1}{r^2}\left(\frac{r^2-14Rr+54R^2}{(r-2R)^7}+\frac{r^2+14Rr+54R^2}{(r+2R)^7}-\frac{2r^2-60R^2}{r^7}\right) \\ & -\frac{A\sigma^6}{37800}\frac{1}{r}\left(\frac{2r-14R}{(r-2R)^7}-7\frac{r^2-14Rr+54R^2}{(r-2R)^8}+\frac{2r+14R}{(r+2R)^7}-\frac{4}{r^6}+7\frac{2r^2-60R^2}{r^8}\right) \\ & +\frac{A}{6}\left(-4\frac{R^2r}{(r^2-4R^2}^{2}-4\frac{R^2}{r^3}+2\frac{r}{r^2-4R^2}-\frac{2}{r}\right) \end{aligned} \tag{2}$$

Next, by dividing by the cross sectional area of a particle we can estimate the effective “van der Waals stress”, as shown in Figure 2. This represents the stress needed to counteract the van der Waals effect and separate two particles.

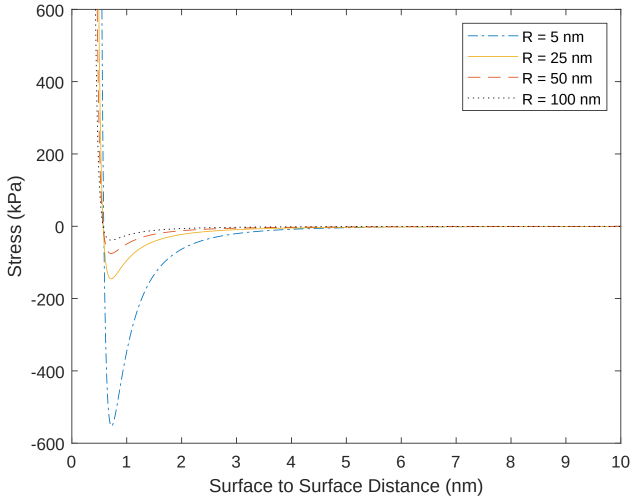


Figure 2: Effective stress generated by the Everaers potential between two spherical particles of radius R and Hamaker constant $1 \times 10^{-19}$ J

Figure 3 displays the stress-strain plot of an Ecoflex silicone with 5 % Carbon Black by weight, and the maximum attractive van der Waals stresses for comparison.

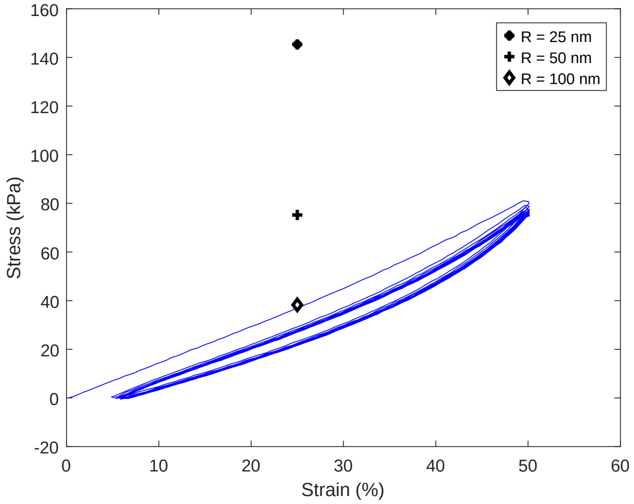


Figure 3: Stress-Strain plot of Ecoflex 0045 + 5wt% Vulcan XC72R Carbon Black, and maximum stress generated by the Everaers potential between two particles of radius $R$ and Hamaker constant $1 \times 10^{-19}$ J

Thus, with reasonable parameter values, it can be seen that the stresses that can be generated by van der Waals interactions are in fact comparable to, and potentially even larger than the average stresses in a composite under large deformation. From this alone, it is clearly plausible that van der Waals interactions may continue to exert an influence on filler network structure even in a cured composite. Lending further credence to this idea is that this is only when comparing the average stress, the actual stress distribution at the scale of the filler particles will fluctuate significantly around this average value. Thus, even materials with lower Hamaker constants may still be influenced by this interaction.

# 2 Full potential energy calculation

## 2.1 Van der Waals and viscoelastic potential energy

The interaction energy between two interacting particles is the sum of the Everaers potential and the viscoelastic potential energy of the linear viscoelastic element between the particles. Both of these can be calculated based on the distance $r$ between the particles. The Everaers potential is directly dependent on $r$, as shown in Equation 1.

The viscoelastic potential energy of a single pair of interacting particles is also dependent on $r$ through the strain $\varepsilon$ of the graph edge:

$$\varepsilon = \frac{r - r_0}{r_0} \tag{3}$$

Where $r_0$ is the initial edge length, defined before any deformation is applied to the system. The linear viscoelastic elements are defined according the Prony series [5]:

$$G(t) = G_\infty + \sum_i G_i \exp\left(\frac{-t}{\tau_i}\right) \tag{4}$$

Where $G$ is the current modulus, $G_\infty$ is the long term modulus, $G_i$ is the modulus of term $i$, and $\tau_i$ is the relaxation time of term $i$. The stress at any moment depends on the entire strain history of the material,

and for discrete timesteps the stress $\sigma$ at timestep $n$ can be calculated as:

$$\sigma_{(n)} = 2G_0 \left( \varepsilon_{(n)} - \sum_i \alpha_i \varepsilon_{i,(n)} \right) \tag{5}$$

Where $\sigma_{(n)}$ is the current stress, $\varepsilon_{(n)}$ is the current strain, $\alpha_i$ is the relative modulus of term $i$, defined as $\alpha_i = \frac{G_i}{G_0}$. $G_0$ is the instantaneous modulus of the material, defined as $G_0 = G_\infty + \sum_i G_i$, and $\varepsilon_i$ is the current viscous strain of term $i$. For discrete timesteps this can be calculated as:

$$\begin{aligned} \varepsilon_{i,(n)} = \varepsilon_{i,(n-1)} &+ \frac{\tau_i}{\Delta t} \left( \frac{\Delta t}{\tau_i} + \exp\left( \frac{-\Delta t}{\tau_i} \right) - 1 \right) (\varepsilon_{(n)} - \varepsilon_{(n-1)}) \\ &+ \left( 1 - \exp\left( \frac{-\Delta t}{\tau_i} \right) \right) (\varepsilon_{(n-1)} - \varepsilon_{i,(n-1)}) \end{aligned} \tag{6}$$

This provides the current stresses for each bond, and the current elastic strain energy density for a linear viscoelastic element is defined as [5]:

$$W_{\text{elastic}} = \frac{1}{2G_0} \sigma_{(n)}^2 \tag{7}$$

The elastic energy $U_{\text{elastic}}$ of the one-dimensional bond with equilibrium length $r_0$ is:

$$U_{\text{elastic}} = W_{\text{elastic}} r_0 \tag{8}$$

The total interaction energy is therefore the sum of the Everaers and viscoelastic potential energies over all bonds.

$$U_{\text{total}} = \sum_i U_i \tag{9a}$$

$$U_i = U_{\text{vdw},i} + U_{\text{elastic},i} \tag{9b}$$

## 2.2 Mapping from seed states to interparticle distances

As described, the discrete, rigid units for these simulations were not individual particles, but rigid collections of particles termed ‘aggregates’, as shown in Figure 4.

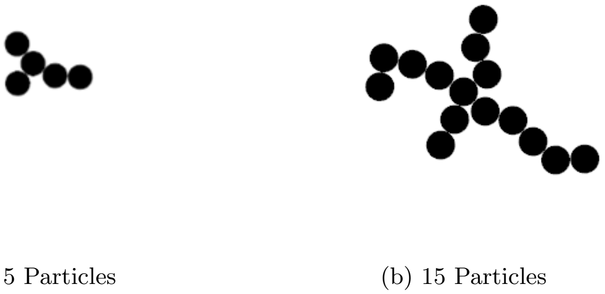

(a) 5 Particles

(b) 15 Particles

Figure 4: Aggregates generated by diffusion limited aggregation

In order to treat these as rigid bodies, a single particle in each aggregate was chosen as the ‘seed’ particle, with a defined position and orientation. All other particles in the aggregate were defined to have a fixed

distance $l$ and relative angle $\phi$ from the seed particle. Thus, the input variables for the energy minimisation were the collection of all seed positions and orientations, termed 'seed states'.

In order to minimize the total potential energy of the interaction network, we need to express the energy as a function of the seed states. These are related by the chain of functions described in Equation 10.

$$U_{total}(\mathbf{s}) = \Sigma \mathbf{U}(\mathbf{r}), \mathbf{r} = \mathbf{r}(\mathbf{d}), \mathbf{d} = \mathbf{d}(\mathbf{x}), \mathbf{x} = \mathbf{x}(\mathbf{s}) \tag{10}$$

Where $U_{total}$ is the total interaction energy as a function of all interparticle distances $\mathbf{r}$, $\mathbf{r}$ is a function of displacements $\mathbf{d}$, $\mathbf{d}$ is a function of particle positions $\mathbf{x}$, and $\mathbf{x}$ is a function of the seed states $\mathbf{s}$.

The NETR algorithm in Scipy requires the state variables to be in the form of a one-dimensional vector. Thus the flattened seed state vector is represented as:

$$s_{3\times k} = \text{x position of seed } k \tag{11a}$$

$$s_{3\times k+1} = \text{y position of seed } k \tag{11b}$$

$$s_{3\times k+2} = \text{orientation angle } \theta \text{ of seed } k \tag{11c}$$

To find the position vector of all particle positions $\mathbf{x}(\mathbf{s})$, we need to know which seed corresponds to each particle. This seed index for each particle is stored in the vector $\mathbf{a}$. Thus the flattened position vector for each particle can be found from:

$$x_{2\times i} = s_{3\times a_i} + l_i \cos(\phi_i + s_{3\times a_i+2}) \tag{12a}$$

$$x_{2\times i+1} = s_{3\times a_i+1} + l_i \sin(\phi_i + s_{3\times a_i+2}) \tag{12b}$$

Where $l_i$ is the distance between particle $i$ and its seed, and $\phi_i$ is the angle between them.

As is common in discrete element simulations, periodic boundary conditions were used for this modelling to approximate the behaviour of a large volume of material. Therefore, all position type variables ($x$, $y$) must always be corrected for periodic boundaries, centred at (0,0), as in Equation 13. $X$ and $Y$ are the x and y lengths of the simulation region.

$$x = \left(\frac{X}{2} + x\right) \bmod (X) - \frac{X}{2} \tag{13a}$$

$$y = \left(\frac{Y}{2} + y\right) \bmod (Y) - \frac{Y}{2} \tag{13b}$$

All displacement type variables ($\Delta x$, $\Delta y$) must use the minimum image convention (Equation 14).

$$\Delta x = \Delta x - \left\lfloor \frac{\Delta x}{X} \right\rceil \cdot X \tag{14a}$$

$$\Delta y = \Delta y - \left\lfloor \frac{\Delta y}{Y} \right\rceil \cdot Y \tag{14b}$$

Interparticle interactions are represented as a graph, with edges representing interactions. The interparticle distances between interacting particles can be found from the particles positions and the incidence matrix $\mathbf{B}$ of the interaction graph. The length of edge $j$ ($r_j$) can be calculated as in Equation 15.

$$\mathbf{d} = \mathbf{B}\mathbf{x} \tag{15a}$$

$$d_{2j} = \Delta x_j,\ d_{2j+1} = \Delta y_j \tag{15b}$$

$$r_j = \sqrt{d_{2j}^2 + d_{2j+1}^2} \tag{15c}$$

## 3 Jacobian (gradient vector) derivation

As the derivations of the derivatives requires higher dimensional tensors, Einstein notation is used for the following calculations. Manual calculation of the derivatives was necessary as numerical approximations were not able to reach a solution in a reasonable amount of time, and automatic differentiation tools available in libraries such as PyTorch are not currently well equipped to handle sparse systems efficiently.

By using the chain rule, we can calculate the derivative of the energy with respect to the seed states:

$$\frac{dU}{ds_i} = \frac{\partial U}{\partial r_j}\frac{\partial r_j}{\partial d_k}\frac{\partial d_k}{\partial x_l}\frac{\partial x_l}{\partial s_i} \tag{16}$$

Each derivative in Equation 16 can be found by differentiating the equations of the previous section.

Differentiating Equation 12:

$$\frac{\partial x_{2i}}{\partial s_j} = \delta_{j,3a_i} - l_i \sin(\phi_i + s_{3a_i+2})\delta_{j,3a_i+2} \tag{17a}$$

$$\frac{\partial x_{2i+1}}{\partial s_j} = \delta_{j,3a_i} + l_i \cos(\phi_i + s_{3a_i+2})\delta_{j,3a_i+2} \tag{17b}$$

Where $\delta_{i,j}$ is the Kronecker delta, equal to 1 if $i = j$, and 0 otherwise.

Differentiating Equation 15:

$$\frac{\partial d_i}{dx_j} = B_{ij} \tag{18}$$

Differentiating Equation 15

$$\frac{\partial r_i}{\partial d_j} = \frac{1}{2\sqrt{d_{2i}^2 + d_{2i+1}^2}}(2d_{2i}\delta_{j,2i} + 2d_{2i+1}\delta_{j,2i+1}) \tag{19}$$

Finally, the total energy is the sum of all bond energies:

$$U_{\text{total}} = \sum_i U_i \tag{20}$$

Thus:

$$\frac{\partial U}{\partial r_j} = \frac{\partial U_i}{\partial r_j}\delta_{j,i} \tag{21}$$

where

$$\frac{\partial U_i}{\partial r_i} = \frac{dU}{dr}(r = r_i) \tag{22}$$

## 4 Hessian calculations

Once again, application of the chain rule gives:

$$\begin{aligned}\frac{\partial^2 U}{\partial s_i \partial s_j} &= \frac{\partial^2 U}{\partial r_k \partial r_q}\frac{\partial r_q}{\partial d_p}\frac{\partial r_k}{\partial d_l}\frac{\partial d_l}{\partial x_m}\frac{\partial d_p}{\partial x_m}\frac{\partial x_m}{\partial s_i}\frac{\partial x_n}{\partial s_j} \\ &+ \frac{\partial^2 r_k}{\partial d_l \partial d_p}\frac{\partial U}{\partial r_k}\frac{\partial d_l}{\partial x_m}\frac{\partial d_p}{\partial x_n}\frac{\partial x_m}{\partial s_i}\frac{\partial x_n}{\partial s_j} \\ &+ \frac{\partial^2 d_l}{\partial x_m \partial x_n}\frac{\partial U}{\partial r_k}\frac{\partial r_k}{\partial d_l}\frac{\partial x_m}{\partial s_i}\frac{\partial x_n}{\partial s_j} \\ &+ \frac{\partial^2 x_m}{\partial s_i \partial s_j}\frac{\partial U}{\partial r_k}\frac{\partial r_k}{\partial d_l}\frac{\partial d_l}{\partial x_m}\end{aligned} \tag{23}$$

The first derivatives have already been found. Each second derivative can be found as follows.

$$\frac{\partial^2 x_i}{\partial s_j \partial s_k} = \frac{\partial}{\partial s_k}\left(\frac{\partial x_i}{\partial sj}\right) \tag{24}$$

$$\begin{aligned}\frac{\partial^2 x_{2i}}{\partial s_j \partial s_k} &= \frac{\partial}{\partial s_k}\left(\delta_{j,3a_i} - l_i \sin(\phi_i + s_{3a_i+2})\delta_{j,3a_i+2}\right) \\ &= -l_i \cos(\phi_i + s_{3a_i+2})\delta_{j,3a_i+2}\delta_{k,3a_i+2}\end{aligned} \tag{25a}$$

$$\begin{aligned}\frac{\partial^2 x_{2i+1}}{\partial s_j \partial s_k} &= \frac{\partial}{\partial s_k}\left(\delta_{j,3a_i} + l_i \cos(\phi_i + s_{3a_i+2})\delta_{j,3a_i+2}\right) \\ &= -l_i \sin(\phi_i + s_{3a_i+2})\delta_{j,3a_i+2}\delta_{k,3a_i+2}\end{aligned} \tag{25b}$$

$$\frac{\partial^2 d_i}{\partial x_j \partial x_k} = \frac{\partial}{\partial x_k}(B_{ij}) = 0 \tag{26a}$$

$$\begin{aligned}\frac{\partial^2 r_i}{\partial d_j \partial d_k} &= \frac{\partial}{\partial d_k}\left(\frac{1}{\sqrt{d_{2i}^2 + d_{2i+1}^2}}(2d_{2i}\delta_{j,2i} + 2d_{2i+1}\delta_{j,2i+1})\right) \\ &= -\frac{1}{4}(d_{2i}^2 + d_{2i+1}^2)^{-\frac{3}{2}}(2d_{2i}\delta_{j,2i} + 2d_{2i+1}\delta_{j,2i+1})(2d_{2i}\delta_{k,2i} + 2d_{2i+1}\delta_{k,2i+1}) \\ &+ \frac{1}{2}(d_{2i}^2 + d_{2i+1}^2)^{-\frac{1}{2}}(2\delta_{j,2i}\delta_{k,2i} + 2\delta_{j,2i+1}\delta_{k,2i+1})\end{aligned} \tag{27a}$$

Finally:

$$\frac{\partial^2 U}{\partial r_j \partial r_k} = \frac{\partial}{\partial r_k}\left(\frac{\partial U_i}{\partial r_j}\delta_{j,i}\right) = \frac{\partial^2 U_i}{\partial r_j \partial r_k}\delta_{j,i}\delta_{k,i} \tag{28}$$

Where

$$\frac{\partial^2 U_i}{\partial r_i \partial r_i} = \frac{d^2 U}{dr^2}(r = r_i) \tag{29}$$

# 5 Everaers and viscoelastic potential derivatives

All that's left is to find the first and second derivatives of the Everaers and viscoelastic potentials with respect to interparticle distance $r$.

## 5.1 Everaers potential

We begin by breaking the full equation into separate parts to differentiate individually.

$$\begin{aligned} U_{vdw} &= U_r + U_a \\ U_r &= \frac{A}{37800r}\left(U_{r1} + U_{r2} + U_{r3}\right) \\ U_A &= -\frac{A}{6}\left(U_{A1} + U_{A2} + U_{A3}\right) \\ U_{r1} &= \frac{r^2 - 14Rr + 54R^2}{(r-2R)^7} \\ U_{r2} &= \frac{r^2 + 14Rr + 54R^2}{r^7} \\ U_{r3} &= -\frac{2r^2 - 60R^2}{r^7} \end{aligned} \tag{30a}$$

$$\begin{aligned} U_{A1} &= \frac{2R^2}{r^2 - 4R2} \\ U_{A2} &= \frac{2R^2}{r^2} \\ U_{A3} &= \ln\left(\frac{r^2 - 4R^2}{r^2}\right) \end{aligned} \tag{30b}$$

The first derivative is therefore:

$$\frac{\partial U_{vdw}}{\partial r} = \frac{\partial U_r}{\partial r} + \frac{\partial U_A}{\partial r} \tag{31a}$$

$$\frac{\partial U_r}{\partial r} = -\frac{A}{37800r^2}(U_{r1} + U_{r2} + U_{r3}) + \frac{A}{37800r}\left(\frac{\partial U_{r1}}{\partial r} + \frac{\partial U_{r2}}{\partial r} + \frac{\partial U_{r3}}{\partial r}\right) \tag{31b}$$

$$\frac{\partial U_{r1}}{\partial r} = \frac{(2r-14R)(r-2R) - 7(r^2 - 14Rr + 54R^2)}{(r-2R)^8} \tag{31c}$$

$$\frac{\partial U_{r2}}{\partial r} = \frac{(2r+14R)(r+2R) - 7(r^2 + 14Rr + 54R^2)}{(r+2R)^8} \tag{31d}$$

$$\frac{\partial U_{r3}}{\partial r} = -\frac{4r^2 - 7(2r^2 - 60R^2)}{r^8} \tag{31e}$$

$$\frac{\partial U_A}{\partial r} = -\frac{A}{6}\left(\frac{\partial U_{A1}}{\partial r} + \frac{\partial U_{A2}}{\partial r} + \frac{\partial U_{A3}}{\partial r}\right) \tag{32a}$$

$$\frac{\partial U_{A1}}{\partial r} = \frac{-4R^2 r}{(r^2 - 4R^2)^2} \tag{32b}$$

$$\frac{\partial U_{A2}}{\partial r} = \frac{-4R^2 r}{r^4} \tag{32c}$$

$$\frac{\partial U_{A3}}{\partial r} = \frac{8R^2}{r^3 - 4R^2} \tag{32d}$$

Differentiating again we calculate the second derivative:

$$\frac{\partial^2 U}{\partial r^2} = \frac{\partial^2 U_r}{\partial r^2} + \frac{\partial^2 U_A}{\partial r^2} \tag{33a}$$

$$\begin{aligned}\frac{\partial^2 U_r}{\partial r^2} &= \frac{2A}{37800r^3}(U_{r1} + U_{r2} + U_{r3}) - \frac{2A}{37800r^2}\left(\frac{\partial U_{r1}}{\partial r} + \frac{\partial U_{r2}}{\partial r} + \frac{\partial U_{r3}}{\partial r}\right) \\ &+ \frac{A}{37800r}\left(\frac{\partial^2 U_{r1}}{\partial r^2} + \frac{\partial^2 U_{r2}}{\partial r^2} + \frac{\partial U_{r3}^2}{\partial r^2}\right)\end{aligned} \tag{33b}$$

$$\frac{\partial^2 U_A}{\partial r^2} = -\frac{A}{6}\left(\frac{\partial^2 U_{A1}}{\partial r^2} + \frac{\partial^2 U_{A1}}{\partial r^2} + \frac{\partial^2 U_{A1}}{\partial r^2}\right) \tag{34a}$$

$$\frac{\partial^2 U_{r1}}{\partial r^2} = \frac{2(r-2R) - 7(2r-14R)}{(r-2R)^8} - \frac{7((2r-14R)(r-2R) - 8(r^2 - 14Rr + 54R^2))}{(r-2R)^9} \tag{35a}$$

$$\frac{\partial^2 U_{r2}}{\partial r^2} = \frac{2(r+2R) - 7(2r+14R)}{(r+2R)^8} - \frac{7((2r+14R)(r+2R) - 8(r^2 + 14Rr + 54R^2))}{(r+2R)^9} \tag{35b}$$

$$\frac{\partial^2 U_{r3}}{\partial r^2} = \frac{24}{r^7} + \frac{7(4r^2 - 8(2r^2 - 60R^2))}{r^9} \tag{35c}$$

$$\frac{\partial^2 U_{A1}}{\partial r^2} = \frac{-4R^2(r^2 - 4R^2) + 16R^2 r^2}{(r^2 - 4R^2)^3} \tag{36a}$$

$$\frac{\partial^2 U_{A2}}{\partial r^2} = \frac{12R^2}{r^4} \tag{36b}$$

$$\frac{\partial^2 U_{A3}}{\partial r^2} = \frac{2(r^2 - 4R^2) - 4r^2}{(r^2 - 4R^2)^2 + \frac{2}{r^2}} \tag{36c}$$

## 5.2 Viscoelastic potential

The first derivative can be found by differentiating Equation 8:

$$U_{\text{elastic}} = \frac{r_0}{2G_0}\sigma_{(n)}^2 \tag{37a}$$

$$\sigma_{(n)} = 2G_0(\varepsilon_{(n)} - \sum_i \alpha_i \varepsilon_{i,(n)}) \tag{37b}$$

$$\varepsilon_{i,(n)} = \varepsilon_{i,(n-1)} + \frac{\tau}{\Delta t}\left(\frac{\Delta t}{\tau} + \exp\left(\frac{-\Delta t}{\tau}\right) - 1\right)(\varepsilon_{(n)} - \varepsilon_{(n-1)}) + \left(1 - \exp\left(\frac{-\Delta t}{\tau}\right)\right)(\varepsilon_{(n-1)} - \varepsilon_{i,(n-1)}) \tag{37c}$$

$$\varepsilon_{(n)} = \frac{r - r_0}{r_0} \tag{37d}$$

$$\frac{dU_{\text{elastic}}}{dr} = \frac{dU}{d\sigma_{(n)}}\frac{d\sigma_{(n)}}{d\varepsilon_{(n)}}\frac{d\varepsilon_{(n)}}{d_r} \tag{38a}$$

$$\frac{dU_{\text{elastic}}}{d\sigma_{(n)}} = \frac{r_0}{G_0}\sigma_{(n)} \tag{38b}$$

$$\frac{d\sigma_{(n)}}{d\varepsilon_{(n)}} = 2G_0 - 2G_0\sum_i \alpha_i \frac{d\varepsilon_{i,(n)}}{d\varepsilon_{(n)}} \tag{38c}$$

$$\frac{d\varepsilon_{i,(n)}}{d\varepsilon_{(n)}} = \frac{\tau}{\Delta t}\left(\frac{\Delta t}{\tau} + \exp\left(\frac{-\Delta t}{\tau}\right) - 1\right) \tag{38d}$$

$$\frac{d\varepsilon_{(n)}}{dr} = \frac{1}{r_0} \tag{38e}$$

Differentiating again yields the second derivative:

$$\frac{d^2U_{\text{elastic}}}{dr^2} = \frac{d^2U_{\text{elastic}}}{d\sigma_{(n)}^2}\left(\frac{d\sigma_{(n)}}{d\varepsilon_{(n)}}\right)^2\left(\frac{d\varepsilon_{(n)}}{dr}\right)^2 + \frac{d^2\sigma_{(n)}}{d\varepsilon_{(n)}^2}\frac{dU_{\text{elastic}}}{d\sigma_{(n)}}\left(\frac{d\varepsilon_{(n)}}{dr}\right)^2 + \frac{d^2\varepsilon_{(n)}}{dr^2}\frac{dU_{\text{elastic}}}{d\sigma_{(n)}}\frac{d\sigma_{(n)}}{d\varepsilon_{(n)}} \tag{39a}$$

$$\frac{d^2U_{\text{elastic}}}{d\sigma_{(n)}^2} = \frac{r_0}{G_0} \tag{39b}$$

$$\frac{d^2\sigma_{(n)}}{d\varepsilon_{(n)}^2} = 0 \tag{39c}$$

$$\frac{d^2\varepsilon_{(n)}}{dr^2} = 0 \tag{39d}$$

# References


[1] R. Everaers and M. R. Ejtehadi. Interaction potentials for soft and hard ellipsoids. *Phys. Rev. E*, 67:041710, Apr 2003.

[2] Saeed Khodabakhshi, Pasquale F. Fulvio, and Enrico Andreoli. Carbon black reborn: Structure and chemistry for renewable energy harnessing. *Carbon*, 162:604–649, 2020.

[3] Raymond R. Dagastine, Dennis C. Prieve, and Lee R. White. Calculations of van der waals forces in 2-dimensionally anisotropic materials and its application to carbon black. *Journal of Colloid and Interface Science*, 249(1):78–83, 2002.

[4] H.C. Hamaker. The london—van der waals attraction between spherical particles. *Physica*, 4(10):1058–1072, 1937.

[5] Dassault Systemes. *Abaqus 2024 Theory Guide*, 2024.
